# Supplementary material for: From Data to Insights: A Covariate Analysis of the IARPA BRIAR Dataset for Multimodal Biometric Recognition Algorithms at Altitude and Range
Source: arXiv:2409.01514 source file (2024-09-03)
Supplement: Supplementary file 1 [file supplimental.tex]

\newpage

%------------------------------------------------------------------------
\section*{Supplemental Material}

\begin{table*}[h]
    \centering
\begin{tabular}{lllll}
\hline
algorithm tag & developer & name & version & results \\
\hline
System A & Systems Technology Research & Str Morfius & 2.2.3 &  \\
System B & Michigan State University & humanid & 3.8.1 &  \\
System C & Kitware & Kitware DOERS BRIAR Service & 2.1.0 &  \\
System D & Accenture Federal Services & AFSBLAU & 2.9.3 &  \\
System E & University of Southern California & GrailService.v2.0 & 2.0.0 &  \\
\hline
\end{tabular}
    \caption{Caption}
    \label{tab:my_label}
\end{table*}

\begin{table*}[h]
    \centering
\begin{tabular}{ll}
\hline
Evaluation Protocol Summary &  \\
\hline
Evaluation Protocol Version & 4.2.1 \\
Evaluation Phase & 2 \\
Probe Set & main \\
Gallery Type & simple \\
\hline
\end{tabular}

    \caption{Caption}
    \label{tab:my_label}
\end{table*}

\begin{table*}[h]
    \centering
\begin{tabular}{lllll}
\hline
 & 0 & 1 & 2 & 3 \\
\hline
0 & Model: & MixedLM & Dependent Variable: & est far \\
1 & No. Observations & 41119 & Method & REML \\
2 & No. Groups: & 55 & Scale: & 4.3539 \\
3 & Min. group size: & 30 & Log-Likelihood: & -88768.7911 \\
4 & Max. group size: & 3185 & Converged: & Yes \\
5 & Mean group size: & 747.6 &  &  \\
\hline
\end{tabular}
    \caption{Caption}
    \label{tab:my_label}
\end{table*}

\begin{table*}
    \centering
\begin{tabular}{lllllll}
\hline
Cov.Name & Level & Coef. & [0.025 & 0.975] & P>|z| & Num.Probes \\
\hline
Intercept & - & -7.003 & -7.340 & -6.666 & 0.000 & - \\
Algorithm & System A & 0.000000 & 0 & 0 & - & 8245 \\
Algorithm & System B & 0.273 & 0.210 & 0.337 & 0.000 & 8213 \\
Algorithm & System C & 0.447 & 0.383 & 0.511 & 0.000 & 8230 \\
Algorithm & System D & 0.692 & 0.628 & 0.756 & 0.000 & 8237 \\
Algorithm & System E & 0.407 & 0.343 & 0.471 & 0.000 & 8194 \\
Has Gait & False & 0.000000 & 0 & 0 & - & 24804 \\
Has Gait & True & -0.283 & -0.332 & -0.233 & 0.000 & 0 \\
Has Turb. & False & 0.000000 & 0 & 0 & - & 27586 \\
Has Turb. & True & 0.057 & -0.012 & 0.127 & 0.104 & 0 \\
Head Height & >90 Pix & 0.000000 & 0 & 0 & - & 11388 \\
Head Height & 60-90 Pix & 0.480 & 0.384 & 0.576 & 0.000 & 3473 \\
Head Height & 50-60 Pix & 0.516 & 0.406 & 0.625 & 0.000 & 3293 \\
Head Height & 40-50 Pix & 0.673 & 0.576 & 0.771 & 0.000 & 7253 \\
Head Height & 30-40 Pix & 1.322 & 1.216 & 1.428 & 0.000 & 4581 \\
Head Height & <30 Pix & 1.884 & 1.730 & 2.038 & 0.000 & 1290 \\
Head Height & Restricted & 2.232 & 2.151 & 2.313 & 0.000 & 9841 \\
Modality & Face & 0.000000 & 0 & 0 & - & 10525 \\
Modality & Body & 0.742 & 0.642 & 0.842 & 0.000 & 30594 \\
Camera Location & Ctrl & 0.000000 & 0 & 0 & - & 7392 \\
Camera Location & Short Range & -0.344 & -0.489 & -0.200 & 0.000 & 2155 \\
Camera Location & Medium Range & 0.949 & 0.792 & 1.106 & 0.000 & 10472 \\
Camera Location & Long Range & 1.952 & 1.716 & 2.187 & 0.000 & 9673 \\
Camera Location & Elevated & 0.214 & 0.109 & 0.318 & 0.000 & 10510 \\
Camera Location & Uav & 0.999 & -0.122 & 2.120 & 0.081 & 917 \\
Solar Loading & 0-300 W/M$^2$ & 0.000000 & 0 & 0 & - & 19375 \\
Solar Loading & 300-600 W/M$^2$ & -0.199 & -0.266 & -0.132 & 0.000 & 7404 \\
Solar Loading & 600-900 W/M$^2$ & 0.511 & 0.434 & 0.588 & 0.000 & 7024 \\
Solar Loading & Above 900 W/M$^2$ & 0.868 & 0.791 & 0.945 & 0.000 & 7316 \\
Wind Speed & 0-3 M/S & 0.000000 & 0 & 0 & - & 25929 \\
Wind Speed & 3-6 M/S & -0.156 & -0.213 & -0.099 & 0.000 & 12453 \\
Wind Speed & 6-9 M/S & -0.043 & -0.145 & 0.059 & 0.412 & 2432 \\
Wind Speed & 9-12 M/S & 0.265 & 0.013 & 0.516 & 0.039 & 305 \\
Temperature & Below 0 C & 0.000000 & 0 & 0 & - & 4059 \\
Temperature & 0-10 C & 0.114 & 0.031 & 0.197 & 0.007 & 8327 \\
Temperature & 10-20 C & 0.333 & 0.185 & 0.481 & 0.000 & 8178 \\
Temperature & 20-30 C & -0.342 & -0.501 & -0.183 & 0.000 & 17684 \\
Temperature & 30-40 C & -0.143 & -0.329 & 0.043 & 0.132 & 2871 \\
Group Var & - & 1.157 &  &  &  & - \\
\hline
\end{tabular}

    \caption{Caption}
    \label{tab:my_label}
\end{table*}

\begin{table*}
    \centering

\begin{tabular}{lr}
\hline
 & count \\
group &  \\
\hline
DWC-MPTZ336XW - BGC3 & 3185 \\
acA2040-90um - BGC4 & 2175 \\
DWC-MPTZ336XW - BGC1 & 2025 \\
HDZP252DI - BGC3 & 1875 \\
acA2040-120uc - BGC2 & 1601 \\
XNZ-6320 - BGC3 & 1591 \\
acA2040-120uc - BGC1 & 1535 \\
HDZP252DI - BGC1 & 1490 \\
MPT-50 - BGC4 & 1465 \\
acA2040-120uc - BGC4 & 1429 \\
Q6215-LE - BGC4 & 1427 \\
PNP-9200RH - BGC2 & 1315 \\
HDZP252DI - BGC2 & 1303 \\
HDZP252DI - BGC4 & 1182 \\
MPT-90 - BGC2 & 1074 \\
acA2040-120um - BGC2 & 1060 \\
PNP-9200RH - BGC3 & 1055 \\
DWC-MPTZ336XW - BGC2 & 965 \\
acA2040-120uc - BGC3 & 911 \\
acA4112-30um - BGC4 & 848 \\
acA4112-30um - BGC3 & 771 \\
XNZ-6320 - BGC4 & 733 \\
XNZ-6320 - BGC2 & 721 \\
Q6215-LE - BGC2 & 680 \\
acA2040-90um - BGC2 & 644 \\
acA4112-30um - BGC1 & 610 \\
PNP-9200RH - BGC1 & 605 \\
Q6215-LE - BGC3 & 525 \\
Q6215-LE - BGC1 & 505 \\
QNP-6230H - BGC3 & 480 \\
P5655-E - BGC4 & 470 \\
Anafi - BGC1 & 465 \\
QNP-6230H - BGC4 & 450 \\
DWC-MPTZ336XW - BGC1.1 & 420 \\
HDZP252DI - BGC1.1 & 370 \\
P5655-E - BGC2 & 365 \\
XNZ-6320 - BGC1.1 & 284 \\
DWC-MPTZ336XW - BGC4 & 275 \\
Anafi USA - BGC1 & 250 \\
acA2040-90uc - BGC1 & 245 \\
MIC-IP-FUSION-9000IV - BGC4 & 220 \\
MPT-90 - BGC3 & 205 \\
PNP-9200RH - BGC4 & 195 \\
Anafi USA - BGC1.1 & 172 \\
Q6215-LE - BGC1.1 & 170 \\
PNP-9200RH - BGC1.1 & 165 \\
acA2040-120um - BGC1.1 & 123 \\
MIC-IP-FUSION-9000IV - BGC2 & 105 \\
P5655-E - BGC3 & 75 \\
acA2040-120um - BGC3 & 75 \\
P5655-E - BGC1.1 & 65 \\
acA2040-120uc - BGC1.1 & 55 \\
acA2040-90uc - BGC1.1 & 50 \\
a2A5328-15ucPRO - BGC3 & 35 \\
Mantis i45 EO - BGC1.1 & 30 \\
\hline
\end{tabular}

    \caption{Caption}
    \label{tab:my_label}
\end{table*}
